# Supplementary material for: sZoom: A Framework for Automatic Zoom into High Resolution Surveillance Videos
Source: arXiv:1909.10164 source file (2019-09-23)
Supplement: Supplementary file 1 [file additional-papers.tex]

\section{Additional Papers}  
In this section we provide a tabular comparison of our work with previous works. First we highlight the differences, and then we state how these difference make us better.

Ascendent Video Analysis: vision-based company offering products for target counting, intrusion detection, object classification, abondened baggage detection, dwelling etc.

In \cite{gaddam2015cameraman}, the authors automatiz zoom for  panoramic sports video. The RoI is determined on tracking the ball or selected player. The framework is not application for surveillance because: (1) we do not know what to track in advance (2) coverage and context are important which are ignored (3) The RoI adaptation is necessary for natural viewing which is missing (4) no fusion framework.

In \cite{chen2016learning}, the authors use recurrent decision trees for smooth trajectory prediction in sports videos. The smooth trajectory reduces jitter in the automatic camera motion.   

In \cite{wang2015wireless}, the authors propose multicast framework for zoomable video. The work is useful in our framework to extend to multiple users. The RoI is manually selected by the users and there is no automatic zoom. 

In \cite{zhai2015object}, the authors propose object detection by analyzing dense trajectories. It can be integrated easily in our sensitivity detection framework. 

In \cite{lim2014isurveillance}, the authors detect multiple events in different RoIs of the video. This work could be used to adapt the zoom time window (which is currently 5 second) according to the type of event. As the current automatic zoom is aimed to assist the security operator, we detect RoI based on low-level processing and leave the high level understanding to the operator. 

In \cite{zhu2012face} and \cite{li2015convolutional} the authors propose more robust face detection algorithms. Although the accuracy of face detector is very low in current framework, with the new advanced detectors the accuracy would increase. 

In \cite{pang2011classx}, the authors propose a framework to stream video lectures to mobile devices. The user can pan/tilt/zoom onto the streamed video. Once an RoI se selected y the user, the system tracks the RoI in the video until the user selected another RoI. There is not automatic zoom. 

In \cite{carlier2011combining}, the authors use saliency and motion to estimate the regions containing humans. We directly use human detector. Once RoI is detected, the authors recommend the RoI to the user. There is no automatic zoom. sZoom framework is modular in the sense new content analysis techniques can be easily plugged in the fusion step.

In \cite{shafiei2012jiku}, the Jiku live allows user to manually zoom and pan into the real-time video. This is not sufficient for surveillance because, once zoomed in, the user cannot see other parts of video which may contain  sensitive activities going on. Also, it is tiring to continuously keep zooming into different regions using finger gestures. The work does not propose any automatic zoom framework. 

In \cite{koccberber2014video}, the authors crop certain region of the video based on visual saliency and motion. The goal is video retargetting, no automatic zoom framework proposed.
